# Supplementary material for: Bootstrapping Reinforcement Learning with Imitation for Vision-Based Agile Flight
Source: arXiv:2403.12203 source file (2024-11-12)
Supplement: Supplementary file 1 [file drone_params.tex]

\begin{table}[b] 
   \centering 
    \fontsize{9pt}{12pt}\selectfont
            % \begin{subfigure}[t]{0.4\textwidth}
            %      \captionsetup{labelformat=empty}
            %      \caption{\textbf{Agilicious platform}}
            %      \includegraphics[width=1\linewidth]{images/4s.png}
            % \end{subfigure}
    \begin{tabular}{ l | c }
        \toprule
          \textbf{Parameters}  & \textbf{Agilicious platform}  \\ \cline{1-2}
          Thrust-to-weight Ratio   & 5.78  \\
          Mass [\SI{}{\kilogram}]   &    0.6\\
          Maximum Thrust [\SI{}{\newton}]  & 34.00   \\
          Arm Length [\SI{}{\meter}]  & 0.15 \\
          Inertia  [\SI{}{\gram\square\meter}]  & [2.50, 2.51, 4.32] \\
          Motor Time Constant [\SI{}{\second}]  & 0.033 \\ \toprule
         \textbf{Components}  & \textbf{Agilicious platform}  \\ \hline
          Frame &Chameleon 6 inch\\
          Motor & Xrotor 2306 \\
          Propeller & Azure Power SFP 5148 5 \\
          Flight Controller & BrainFPV radix \\
          Battery & Tattu 4 cells 1800 mAh   \\
          Electronic Speed Controller (ESC) &  Hobbywing XRotor \\ 
        \bottomrule
    \end{tabular}
   \vspace{0.5em} 
   \caption{Overview of the drone parameters for real-world experiments.} 
   \label{tab:physical_drone}
\end{table}
